# Supplementary material for: SelfGNN: Self-Supervised Graph Neural Networks for Sequential Recommendation
Source: arXiv:2405.20878 source file (2024-05-31)
Supplement: Supplementary file 1 [file appendix.tex]

\appendix \section{Appendix}
\balance
\label{sec:appendix}
\subsection{Main Notations}
 Table \ref{tab:notations} provides a detailed explanation of the key notations in Figure \ref{fig:overall} and Figure \ref{fig:ssl}.

\begin{table}[H]
\centering
% \small
\footnotesize
\caption{Descriptions of Key Notations.}
\setlength{\tabcolsep}{0.6mm}
\begin{tabular}{|c|c|}
\hline
Notation                             & Description                                                                                               \\ \hline
$u_i$,$v_j$                                           & The ($i$)-th user, the ($j$)-th item                                                                                                         \\ \hline
$\mathcal{G}$                                         & Short-term graph                                                                                                                             \\ \hline
$\mathcal{A}_t$                                       & The adjacent matrix in the ($t$)-th period                                                                                                   \\ \hline
$\hat{\mathcal{A}}_{T+1}$                                       & \begin{tabular}[c]{@{}c@{}}The adjacent matrix for a future time period \\ predicted by \model \end{tabular}                                                                         \\ \hline
$\textbf{E}_t^{(v)}$                                  & Embedding matrices for all items in the ($t$)-th period                                                                                      \\ \hline
${\mathbf{z}_{t,j}^{(v)}}$                            & \begin{tabular}[c]{@{}c@{}}The information aggregated from neighboring nodes \\ to $v_j$\end{tabular}                                        \\ \hline
$\textbf{e}_{t,i}^{(u)}$,$\textbf{e}_{t,j}^{(v)}$     & \begin{tabular}[c]{@{}c@{}}The embedding vector for $u_i$ and $v_j$ in the ($t$)-th \\ period\end{tabular}                                   \\ \hline
$v_{i,m}$                                             & The ($m$)-th interacted item of user $u_i$                                                                                                   \\ \hline
$\tilde{\textbf{e}}_i^{(u)}$                          & \begin{tabular}[c]{@{}c@{}}Feature vector for user $u_i$ with instance-level \\ sequential correlations\end{tabular}                         \\ \hline
$\bar{\textbf{e}}_i^{(u)}, \bar{\textbf{e}}_j^{(v)}$  & \begin{tabular}[c]{@{}c@{}}Feature vectors for $u_i$ and $v_j$ derived from \\ interval-level pattern learning\end{tabular}                  \\ \hline
$\mathcal{L}_{sal}$                                   & Loss function for self-augmented learning                                                                                                    \\ \hline
$\mathcal{L}_{rec}$                                   & Loss function for prediction in recommendation                                                                                               \\ \hline
$s_{t,i,j}$                                           & \begin{tabular}[c]{@{}c@{}}The likelihood of $u_i$ interacting with $v_j$ in the $t$-th \\ period\end{tabular}                               \\ \hline
$\bar{s}_{i,j}$                                       & The likelihood of $u_i$ interacting with $v_j$ in long term                                                                                  \\ \hline
$\mathbf{W}_1$, $\mathbf{W}_2$, $\mathbf{b}_1$, $b_2$ & \begin{tabular}[c]{@{}c@{}}Trainable transformation parameters in personalized \\ weights\end{tabular}                                       \\ \hline
$\sigma$                                              & LeakyReLu function                                                                                                                           \\ \hline
$\rm{sigm}$                                           & Sigmoid function                                                                                                                             \\ \hline
$w_{t, i}$                                            & \begin{tabular}[c]{@{}c@{}}Personalized weights for user $u_i$ in the $t$-th \\ period\end{tabular}                                          \\ \hline
$d_1$                                                 & \begin{tabular}[c]{@{}c@{}}The difference in long-term likelihood values for two \\ user-item pairs with personalized weighting\end{tabular} \\ \hline
$d_2$                                                 & \begin{tabular}[c]{@{}c@{}}The difference in short-term likelihood values for \\ two user-item pairs\end{tabular}                            \\ \hline
                            
\end{tabular}
\label{tab:notations}
\end{table}

\subsection{Model Complexity Analyses}
The short-term GNN encoding takes $\sum_{t=0}^{T}O(L\times |\mathcal{A}_t|\times d)=O(L \times |\mathcal{A}|\times d)$ complexity, where $T$ is the number of short periods divided, $L$ is the layer number of GNN and $|\mathcal{A}|$ is the number of edges in the complete long-term user-item graph. Additionally, the temporal attention-based short-term feature fusion module takes $O((T \times d^2 + T^2 \times  d) \times (I+J))$ complexity, as well as the time complexity in long-term user behavior sequence modeling based on attention is $O((M \times d^2 + M^2 \times  d) \times B)$, where $I$ and $J$ represent the number of users and items respectively and $B$ is the batch size. In our personalized self-augmented learning paradigm, denoting $B_{sal}$ as the batch size of the sample pairs in self-augmented learning, the cost is $O(B_{sal} \times d)$. Comparing our self-augmented learning architecture with the self-supervised learning paradigm in several state-of-the-art approaches, we only need to do a simple vector dot product of randomly selected edges, instead of doing complex operations such as InfoNCE \cite{Oord_2018} loss for all nodes, which greatly reduces the time cost of operations.
\subsection{Hyperparameter Analysis (RQ4)}
In this section, we supplement experiments on the hyperparameter $N_{sal}$, which means the number of edge samples per user in self-augmented learning. 
\begin{figure}[h]
%\vspace{-0.05in}
    \centering
    \begin{adjustbox}{max width=1.0\linewidth}
    \input{./figure/hyper3.tex}
    \end{adjustbox}
    \vspace{-0.2in}
    \caption{Hyperparameter study of the \model.}
    \vspace{-0.1in}
    \label{fig:hyperparam2}
\end{figure}

As depicted in Figure \ref{fig:hyperparam2}, the optimal number of randomly sampled pairs for each user's interaction edges in self-augmented learning varies across different datasets. The densest dataset, Movielens, requires a larger number of samples per user, with 100 pairs being the optimal value. On the other hand, the sparsest dataset, Gowalla, achieves optimal results with 40 sampled pairs per user.
\subsection{Case Study (RQ5)}
As shown in Figure \ref{fig:casestudy2}, we randomly selected a user (48) and part of the behavior sequence of that user, and the other user (226) which has at least 20 interaction items in common with the user (48). 

\begin{figure}[h]
    \centering
    \includegraphics[width=0.40\textwidth]{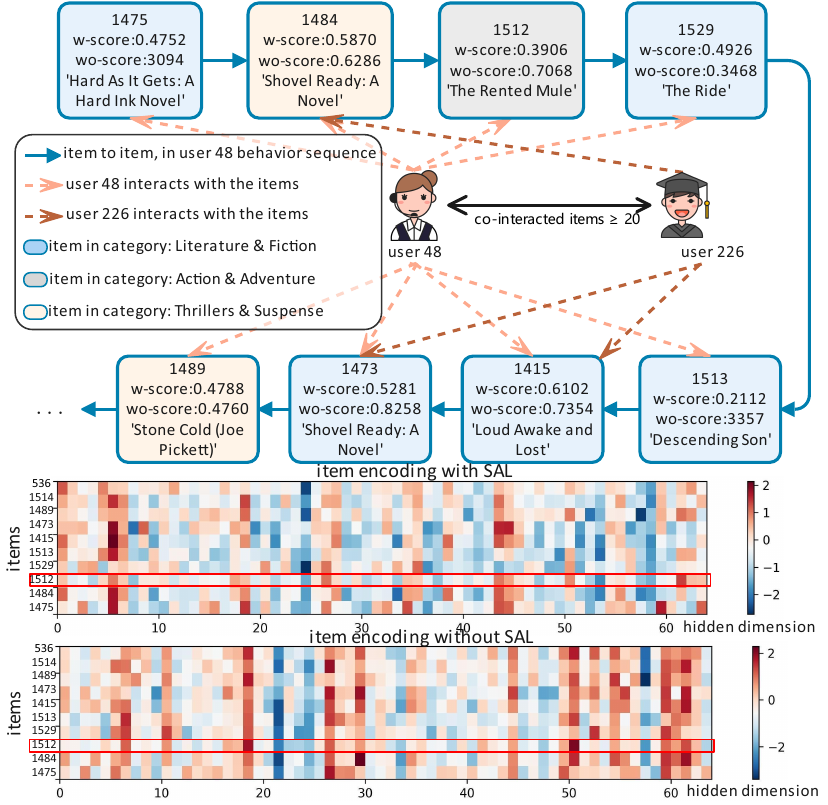}
    \caption{User-item similarity scores in a partial behavior sequence of a user (48) and heatmap of these items' embedding with and without self-augmented learning in \model. }
    \vspace{-5pt}
    \label{fig:casestudy2}
\end{figure}

In Figure \ref{fig:casestudy2}, we can see that for item (1512), self-augmented learning dropped its score from 0.7068 to 0.3906. There are several ways to justify the item needing to be weakened. On the one hand, the category of item (1512) is "Action and Adventure", which is different from the category of other items ("Literature and Fiction" and "Thrillers and Suspense") that the user follows. In addition, as a user with a large number of similar interests with user (48), user (226) does not follow item (1512). In addition, from the perspective of the encoding heatmap of items, the self-augmented learning weakens the values of each dimension of the vector of item (1512), and on the whole also makes the features between the items continuously interacted by the same user more different than without self-augmented learning, which lightens the smoothing problem caused by GNNs.
